# Supplementary material for: Progressively Efficient Learning
Source: arXiv:2310.13004 source file (2023-10-13)
Supplement: Supplementary file 1 [file a4_goal_distribution.tex]

\section{Additional visualization of proposed intention distributions}
In \autoref{s6:results}, we present the visualization of the distribution of intentions proposed by the agent over time for task BakePork. 
in this section, we provide additional visualization for the BakeBeef and SmeltSilver tasks withinin the skill adaptation setting.
